# Supplementary material for: Low-scaling GW algorithm applied to twisted transition-metal dichalcogenide heterobilayers
Source: arXiv:2306.16066 ancillary file (2023-06-28)
Supplement: Supplementary file 1 [file SI.pdf]

## Supporting Information to

### ”Low-scaling $GW$ algorithm applied to twisted transition-metal dichalcogenide heterobilayers”

Maximilian Graml,<sup>1,2</sup> Klaus Zollner,<sup>1</sup> Daniel Hernangómez-Pérez,<sup>3</sup> Paulo E. Faria Junior,<sup>1</sup> and Jan Wilhelm<sup>1,2,\*</sup>

<sup>1</sup>*Institute of Theoretical Physics, University of Regensburg, 93053 Regensburg, Germany*

<sup>2</sup>*Regensburg Center for Ultrafast Nanoscopy (RUN), University of Regensburg, 93053 Regensburg, Germany*

<sup>3</sup>*Department of Molecular Chemistry and Materials Science,  
Weizmann Institute of Science, Rehovot 7610001, Israel*

(Dated: June 28, 2023)

We present the whole  $GW$  algorithm in detail (Sec. S1) and the computational parameters underlying our calculations (Sec. S2). The regularized resolution of the identity used in the  $GW$  algorithm is defined (Sec. S3). We further show the numerical convergence of our benchmark monolayer band gaps (Sec. S4, S5). We discuss the resolution of the identity with the truncated Coulomb metric in Sec. S6. We compare the periodic, low-scaling  $GW$  algorithm from the manuscript to a  $GW$  algorithm with standard scaling (Sec. S7). We also report the number of required floating point operations in our algorithm and in plane-wave algorithms (Sec. S8, S9, S10). Timings of our algorithm are reported in Sec. S11.

#### S1. WORKING EQUATIONS OF THE PERIODIC LOW-SCALING $GW$ ALGORITHM

The  $GW$  algorithm presented in this work starts from a density functional theory (DFT) calculation,

$$\hat{h}_{\text{KS}}(\mathbf{k})\psi_{n\mathbf{k}}(\mathbf{r}) = \varepsilon_{n\mathbf{k}}\psi_{n\mathbf{k}}(\mathbf{r}) \quad (\text{S1})$$

where  $\varepsilon_{n\mathbf{k}}$  are the eigenvalues of the Kohn-Sham Hamiltonian  $\hat{h}_{\text{KS}}(\mathbf{k})$ . Bloch orbitals  $\psi_{n\mathbf{k}}$  are expanded in Gaussians,<sup>1</sup>

$$\psi_{n\mathbf{k}}(\mathbf{r}) = \sum_{\mu} C_{n\mu}(\mathbf{k}) \sum_{\mathbf{R}} e^{i\mathbf{k}\cdot\mathbf{R}} \phi_{\mu}^{\mathbf{R}}(\mathbf{r}), \quad (\text{S2})$$

where the molecular orbital coefficients  $C_{\mu n}$  are optimized in DFT and  $\phi_{\mu}^{\mathbf{R}}$  are Gaussian-type basis functions being centered on an atom in cell  $\mathbf{R}$ .

Following the  $GW$  space-time method<sup>2</sup>, we compute the Green’s function in imaginary time at the  $\Gamma$ -point,<sup>3</sup>

$$G_{\mu\nu}(\mathbf{k}=\mathbf{0}, i\tau) = -\theta(-\tau) \sum_i^{\text{occ}} C_{i\mu}(\mathbf{k}=\mathbf{0}) C_{i\nu}(\mathbf{k}=\mathbf{0}) \exp(-(\varepsilon_i - \varepsilon_F)\tau) + \theta(\tau) \sum_a^{\text{virt}} C_{a\mu}(\mathbf{k}=\mathbf{0}) C_{a\nu}(\mathbf{k}=\mathbf{0}) \exp(-(\varepsilon_a - \varepsilon_F)\tau). \quad (\text{S3})$$

The irreducible polarizability  $\chi_{PQ}(i\tau)$  at  $\mathbf{k}=\mathbf{0}$  in the Gaussian auxiliary basis  $\{\varphi_P^{\mathbf{R}}(\mathbf{r})\}$  follows,<sup>4</sup>

$$\chi_{PQ}(\mathbf{k}=\mathbf{0}, i\tau) = \sum_{\lambda\nu\mu\sigma} (\mu\nu|P) G_{\mu\lambda}(\mathbf{k}=\mathbf{0}, -i\tau) (\lambda\sigma|Q) G_{\nu\sigma}(\mathbf{k}=\mathbf{0}, i\tau) \quad (\text{S4})$$

using three-center matrix elements

$$(\mu\nu|P) = \sum_{\mathbf{R}_1\mathbf{R}_2} \int d\mathbf{r} d\mathbf{r}' \phi_{\mu}^{\mathbf{R}_1}(\mathbf{r}) \phi_{\nu}^{\mathbf{R}_2}(\mathbf{r}) V_{rc}(\mathbf{r}, \mathbf{r}') \varphi_P^{\mathbf{0}}(\mathbf{r}') \quad (\text{S5})$$

of the truncated Coulomb operator

$$V_{rc}(\mathbf{r}, \mathbf{r}') = \begin{cases} 1/|\mathbf{r} - \mathbf{r}'| & \text{if } |\mathbf{r} - \mathbf{r}'| \leq r_c, \\ 0 & \text{else,} \end{cases} \quad (\text{S6})$$

with cutoff radius  $r_c$ . The tensor  $(\mu\nu|P)$  can be understood as deriving from the resolution of the identity with the truncated Coulomb metric (RI-tCm)<sup>4-6</sup> where  $r_c$  is typically chosen to be 3 Å. This choice  $r_c = 3$  Å has been motivated in Refs.<sup>4,6</sup>. We discuss it for the case of periodic  $GW$  in Sec. S6. The locality of  $V_{rc}(\mathbf{r}, \mathbf{r}')$  ensures that the tensor  $(\mu\nu|P)$  is sparsely occupied, making the algorithm computationally efficient. RI-tCm ensures that the resolution of the identity quickly converges with the size of the auxiliary basis  $\{\varphi_P^{\mathbf{R}}(\mathbf{r})\}$ .<sup>4-6</sup> We regularize the RI expansion to prevent linear dependencies of fit coefficients, as we discuss in detail in Sec. S3.

We calculate  $\chi_{PQ}(\mathbf{k}, i\tau)$  for an arbitrary  $k$ -point  $\mathbf{k}$  from the  $\Gamma$ -point result,  $\chi_{PQ}(\mathbf{k}=\mathbf{0}, i\tau)$ , Eq. (S4), as follows: The  $\Gamma$ -point polarizability contains its real-space representations  $\chi_{PQ}^{\mathbf{R}}$ ,

$$\chi_{PQ}(\mathbf{k}=\mathbf{0}, i\tau) = \sum_{\mathbf{R}} \chi_{PQ}^{\mathbf{R}}(i\tau), \quad \chi_{PQ}^{\mathbf{R}} = \langle \varphi_P^0 | \chi | \varphi_Q^{\mathbf{R}} \rangle. \quad (\text{S7})$$

For non-metallic systems,  $G(\mathbf{r}, \mathbf{r}', i\tau)$  is *space-local*, i.e.  $G(\mathbf{r}, \mathbf{r}', i\tau)$  exponentially decays with increasing  $|\mathbf{r} - \mathbf{r}'|$ .<sup>7,8</sup> This locality translates to  $\chi(\mathbf{r}, \mathbf{r}', i\tau) = G(\mathbf{r}, \mathbf{r}', i\tau)G(\mathbf{r}, \mathbf{r}', -i\tau)$ .<sup>2</sup> The matrix representation  $\chi_{PQ}^{\mathbf{R}}$  is thus expected to exponentially decay when increasing the distance between the center of  $\varphi_P^0$  in the unit cell and the center of  $\varphi_Q^{\mathbf{R}}$  in cell  $\mathbf{R}$ . We employ the minimum image convention, i.e., we assume that the contribution  $\chi_{PQ}^{\mathbf{R}}(i\tau)$  in Eq. (S7) is non-zero if and only if the atomic center of  $\varphi_P^0$  and the atomic center of  $\varphi_Q^{\mathbf{R}}$  are closest together among all cells  $\mathbf{R}$ . In this way, we extract  $\chi_{PQ}^{\mathbf{R}}(i\tau)$  from Eq. (S7),

$$\chi_{PQ}^{\mathbf{R}}(i\tau) = \begin{cases} \chi_{PQ}(\mathbf{k}=\mathbf{0}, i\tau) & \text{if } \varphi_P^0, \varphi_Q^{\mathbf{R}} \text{ closest,} \\ 0 & \text{else.} \end{cases} \quad (\text{S8})$$

We transform the irreducible polarizability to  $k$ -space

$$\chi_{PQ}(\mathbf{k}, i\tau) = \sum_{\mathbf{R}} e^{-i\mathbf{k} \cdot \mathbf{R}} \chi_{PQ}^{\mathbf{R}}(i\tau). \quad (\text{S9})$$

and to imaginary frequency,

$$\chi_{PQ}(\mathbf{k}, i\omega) = \int d\tau \cos(\omega\tau) \chi_{PQ}(\mathbf{k}, i\tau). \quad (\text{S10})$$

We have observed that  $\chi_{PQ}(\mathbf{k}, i\omega)$  computed from Eq. (S10) features spurious negative eigenvalues with small absolute value. The reason is most likely that Eq. (S8) together with Eq. (S30) is only exact in the limit of large unit cells. We remove negative eigenvalues from  $\chi_{PQ}(\mathbf{k}, i\omega)$  which requires a costly diagonalization for every  $k$ -point and every frequency point  $\omega$ . Once having a positive definite matrix  $\chi_{PQ}(\mathbf{k}, i\omega)$ , we compute the dielectric function

$$\epsilon(\mathbf{k}, i\omega) = \mathbf{1} - \mathbf{V}^{0.5}(\mathbf{k}) \mathbf{M}^{-1}(\mathbf{k}) \chi(\mathbf{k}, i\omega) \mathbf{M}^{-1}(\mathbf{k}) \mathbf{V}^{0.5}(\mathbf{k}), \quad (\text{S11})$$

where the truncated Coulomb matrix  $\mathbf{M}(\mathbf{k})$  appears due to the RI-tCm,

$$M_{PQ}(\mathbf{k}) = \sum_{\mathbf{R}} e^{-i\mathbf{k} \cdot \mathbf{R}} \int d\mathbf{r} d\mathbf{r}' \varphi_P^0(\mathbf{r}) V_{r_c}(\mathbf{r}, \mathbf{r}') \varphi_Q^{\mathbf{R}}(\mathbf{r}'). \quad (\text{S12})$$

We regularize  $\mathbf{M}^{-1}(\mathbf{k})$  to prevent linear dependencies in the RI expansion, see details in Sec. S3.  $\mathbf{V}^{0.5}(\mathbf{k})$  in Eq. (S12) denotes the square root of the Coulomb matrix<sup>9</sup>

$$V_{PQ}(\mathbf{k}) = \sum_{\mathbf{R}} e^{-i\mathbf{k} \cdot \mathbf{R}} \int d\mathbf{r} d\mathbf{r}' \varphi_P^0(\mathbf{r}) \frac{1}{|\mathbf{r} - \mathbf{r}'|} \varphi_Q^{\mathbf{R}}(\mathbf{r}'). \quad (\text{S13})$$

Eq. (S13) is a lattice sum over Coulomb interactions between charge distributions. The sum will diverge for  $\mathbf{k}=\mathbf{0}$ , if  $\varphi_P$  and  $\varphi_Q$  are  $s$ -type basis functions. We employ even  $k$ -point meshes without  $\mathbf{k}=\mathbf{0}$  to ensure convergence of the lattice sum (S13).

We decompose the screened interaction  $W$  into the truncated Coulomb operator  $V_{r_c}^{\text{HF}}$  used in periodic Hartree-Fock calculations<sup>10</sup> and a correlation part  $W^c$ ,

$$\mathbf{W}(\mathbf{k}, i\omega) = \mathbf{V}_{r_c}^{\text{HF}}(\mathbf{k}) + \mathbf{V}^{0.5}(\mathbf{k}) \left( \epsilon^{-1}(\mathbf{k}, i\omega) - \mathbf{Id} \right) \mathbf{V}^{0.5}(\mathbf{k}). \quad (\text{S14})$$

For the cutoff radius  $r_c^{\text{HF}}$  in Eq. (S14), we set half the minimum of inner box wall distances in periodic directions, which is the common choice in periodic Hartree-Fock calculations<sup>10</sup>. We transform  $W$  to real space,<sup>2</sup>

$$W_{PQ}^{\mathbf{R}}(i\omega) := \langle \varphi_P^0 | W(i\omega) | \varphi_Q^{\mathbf{R}} \rangle = \frac{1}{\Omega_{\text{BZ}}} \int_{\text{BZ}} d\mathbf{k} e^{i\mathbf{k} \cdot \mathbf{R}} W_{PQ}(\mathbf{k}, i\omega), \quad (\text{S15})$$

where  $\Omega_{\text{BZ}}$  is the Brillouin zone (BZ) volume. We discretize the BZ integral in Eq. (S15) using a  $4 \times 4$  and a  $6 \times 6$  Monkhorst-Pack mesh<sup>11</sup> and we extrapolate the BZ integral with the  $k$ -mesh size.<sup>9,12</sup>

We proceed with the calculation of the self-energy  $\Sigma(\mathbf{r}, \mathbf{r}', i\tau) = iG(\mathbf{r}, \mathbf{r}', i\tau)W(\mathbf{r}, \mathbf{r}', i\tau)$ <sup>2</sup>.  $\Sigma(\mathbf{r}, \mathbf{r}', i\tau)$  is space-local as  $G(\mathbf{r}, \mathbf{r}', i\tau)$  is space-local<sup>7</sup> and only elements of  $W(\mathbf{r}, \mathbf{r}', i\tau)$  with small  $|\mathbf{r} - \mathbf{r}'|$  contribute to the  $GW$  self-energy in the Bloch basis. We thus continue with the minimum image of Eq. (S15)

$$W_{PQ}^{\text{MIC}}(i\omega) := W_{PQ}^{\mathbf{R}_{PQ}^{\min}}(i\omega), \quad (\text{S16})$$

where the cell vector

$$\mathbf{R}_{PQ}^{\min} = \underset{\mathbf{R}}{\text{argmin}} |\mathbf{R}_P - (\mathbf{R}_Q + \mathbf{R})| \quad (\text{S17})$$

gives the smallest distance between the atomic centers  $\mathbf{R}_P$  of  $\varphi_P^0$  and the atomic center  $\mathbf{R}_Q + \mathbf{R}$  of  $\varphi_Q^{\mathbf{R}}$ . We include the  $\Gamma$ -point RI metric matrix  $\mathbf{M}$  from Eq. (S12),

$$\tilde{\mathbf{W}}(i\omega) = \mathbf{M}^{-1}(\mathbf{k}=\mathbf{0}) \mathbf{W}^{\text{MIC}}(i\omega) \mathbf{M}^{-1}(\mathbf{k}=\mathbf{0}) \quad (\text{S18})$$

which leads to the self-energy at the  $\Gamma$ -point,

$$\Sigma_{\lambda\sigma}(\mathbf{k}=\mathbf{0}, i\tau) = i \sum_{\nu\mu PQ} (\lambda\mu|Q) G_{\mu\nu}(\mathbf{k}=\mathbf{0}, i\tau) (\nu\sigma|P) \tilde{W}_{PQ}(i\tau). \quad (\text{S19})$$

We obtain  $k$ -points in  $\Sigma$  by MIC, as for  $\chi$  [Eq. (S8), (S10)],

$$\Sigma_{\lambda\sigma}(\mathbf{k}, i\tau) = \sum_{\mathbf{R}} e^{i\mathbf{k}\cdot\mathbf{R}} \cdot \begin{cases} \Sigma_{\lambda\sigma}(\mathbf{k}=\mathbf{0}, i\tau) & \text{if } \phi_{\lambda}^0, \phi_{\sigma}^{\mathbf{R}} \text{ closest,} \\ 0 & \text{else,} \end{cases} \quad (\text{S20})$$

and we transform the self-energy to the Bloch basis,

$$\Sigma_{\mathbf{n}\mathbf{k}}(i\tau) = \sum_{\lambda\sigma} C_{n\lambda}^*(\mathbf{k}) \Sigma_{\lambda\sigma}(\mathbf{k}, i\tau) C_{n\sigma}(\mathbf{k}). \quad (\text{S21})$$

After Fourier transform of  $\Sigma(i\tau)$  to  $\Sigma(i\omega)$ <sup>2-4,13</sup> and analytic continuation to  $\Sigma(\omega)$ <sup>14</sup>, we obtain the quasiparticle energies  $\varepsilon_{n\mathbf{k}}^{G_0W_0}$ ,

$$\varepsilon_{n\mathbf{k}}^{G_0W_0} = \varepsilon_{n\mathbf{k}} + \text{Re} \Sigma_{n\mathbf{k}}(\varepsilon_{n\mathbf{k}}^{G_0W_0}) - v_{n\mathbf{k}}^{\text{xc}}, \quad (\text{S22})$$

where  $v_{n\mathbf{k}}^{\text{xc}}$  is the  $(n, n)$ -diagonal element of the exchange-correlation matrix.

## S2. COMPUTATIONAL DETAILS

The algorithm is implemented in the CP2K software package<sup>15,16</sup>. Unless otherwise noted, we use the TZVP-MOLOPT basis set<sup>15</sup> together with Goedecker-Teter-Hutter pseudopotentials<sup>17</sup> (charge  $q_{\text{Mo}} = q_{\text{W}} = +14e$  and  $q_{\text{S}} = q_{\text{Se}} = +6e$ ). Exemplarily, the TZVP-MOLOPT basis set contains 35 basis functions per Mo atom ( $4 \times s$ ,  $3 \times p$ ,  $3 \times d$ ,  $1 \times f$ ) and 17 basis functions per S atom ( $3 \times s$ ,  $3 \times p$ ,  $1 \times d$ ). As auxiliary basis, we use the relevant exponents from the RI-def2-SVP basis set<sup>18</sup>. Inputs and outputs are available on github<sup>19</sup>. We use a regularized resolution of the identity with regularization parameter  $10^{-2}$ , see Sec. S3 for details.

We use a  $4 \times 4$  and  $6 \times 6$  Monkhorst-Pack  $k$ -point mesh<sup>11</sup> when calculating  $\chi(\mathbf{k})$ ,  $\epsilon(\mathbf{k})$ ,  $V(\mathbf{k})$ ,  $V_{\text{c}}(\mathbf{k})$ ,  $W(\mathbf{k})$ . Using these two  $k$ -meshes, we obtain the numerical values for  $W_{PQ}^{\mathbf{R}}(i\omega)$  in Eq. (S15) by standard extrapolation<sup>9,12</sup> with  $N_k^{-1/d}$ , where  $N_k$  is the number of  $k$ -points and  $d$  is the number of periodic directions. We use an  $8 \times 8$   $k$ -point mesh for the  $GW$  self-energy, Eqs. (S21), (S22). We compute three-center integrals of the truncated Coulomb integrals, Eq. (S5), using the libint library<sup>20</sup>. Two-center integrals are computed using solid harmonic Gaussians<sup>21</sup>. We use minimax grids<sup>13</sup> with ten grid points for the Fourier transform in imaginary time and imaginary frequency. We remove spurious negative eigenvalues and associated eigenvectors from  $\mathbf{M}(\mathbf{k})$  and  $\chi(\mathbf{k}, i\omega)$  to avoid problems in matrix inversions [Eq. (S11), (S14)]. Sparse matrix-tensor operations as in Eqs. (S4), (S19) appear routinely in low-scaling quantum-chemical methods. We employ the dbcsr tensor library<sup>22,23</sup> to execute parallel sparse matrix-tensor operations.

For the plane-wave code benchmarks, the DFT calculations were performed using the QUANTUM ESPRESSO package<sup>24</sup>, with the PBE exchange-correlation functional<sup>25</sup> and norm-conserving non-relativistic pseudopotentials<sup>26</sup>. A basis cut-off of 100 Ry was employed, and the self-consistent charge density was converged on a  $30 \times 30 \times 1$   $\mathbf{k}$ -grid with a total energy accuracy of  $10^{-9}$  Ry. To determine the quasi-particle band-gap, a one-shot  $GW$  calculation ( $G_0W_0$ ) was conducted using the BerkeleyGW package<sup>27,28</sup>. The QUANTUM ESPRESSO DFT converged energies and Kohn-Sham states were used as the starting point. The dielectric matrix was computed with a dielectric cut-off of 25 Ry, considering a total of 1999 occupied and empty bands on a  $12 \times 12 \times 1$  uniform  $\mathbf{k}$ -grid. For the explicit full-frequency calculation, we employed the contour-deformation method with the Adler-Wiser formula. In order to accelerate convergence near the  $\Gamma$ -point ( $|\mathbf{q}| \rightarrow 0$ ), a non-uniform neck subsampling approach was also considered<sup>29</sup>. The spurious interactions between periodic replicas in the perpendicular direction to the surface were removed with a Coulomb interaction truncation scheme<sup>30</sup>.

The heterobilayers were created with the CellMatch code<sup>31</sup>, implementing the coincidence lattice method<sup>32,33</sup>.

### S3. REGULARIZED RESOLUTION OF THE IDENTITY

In this section, we describe the regularization method in the resolution of the identity (RI) that we use in the *GW* algorithm. We show that the regularization accelerates the convergence of the *GW* bandgap with the supercell size.

RI starts from four-center Coulomb integrals (4c-CI)<sup>34</sup>,

$$(\phi_\mu\phi_\nu|\phi_\lambda\phi_\sigma) := \int d\mathbf{r} d\mathbf{r}' \phi_\mu(\mathbf{r}) \phi_\nu(\mathbf{r}) \frac{1}{|\mathbf{r} - \mathbf{r}'|} \phi_\lambda(\mathbf{r}') \phi_\sigma(\mathbf{r}'), \quad (\text{S23})$$

where  $\phi_\mu, \phi_\nu, \phi_\lambda$  and  $\phi_\sigma$  are atomic-orbital (AO) Gaussian basis functions. In RI, one expands the Gaussian products  $\phi_\mu(\mathbf{r})\phi_\nu(\mathbf{r})$  and  $\phi_\lambda(\mathbf{r}')\phi_\sigma(\mathbf{r}')$  using an auxiliary basis  $\{\varphi_P(\mathbf{r})\}$ ,

$$\phi_\mu(\mathbf{r})\phi_\nu(\mathbf{r}) = \sum_P B_{\mu\nu}^P \varphi_P(\mathbf{r}). \quad (\text{S24})$$

$B_{\mu\nu}^P$  are expansion coefficients that will be chosen to approximate  $\phi_\mu(\mathbf{r})\phi_\nu(\mathbf{r})$ . RI is used together with a metric  $m(\mathbf{r}, \mathbf{r}')$ ,<sup>4,5,34</sup> for example the Coulomb metric,  $m(\mathbf{r}, \mathbf{r}') = 1/|\mathbf{r} - \mathbf{r}'|$  or the overlap metric  $m(\mathbf{r}, \mathbf{r}') = \delta(|\mathbf{r} - \mathbf{r}'|)$ . The expansion coefficients  $B_{\mu\nu}^P$  depend on  $m(\mathbf{r}, \mathbf{r}')$  and are chosen, such that the following expression gets minimal:<sup>34</sup>

$$\left( \phi_\mu\phi_\nu - \sum_P B_{\mu\nu}^P \varphi_P \middle| \phi_\lambda\phi_\sigma - \sum_P B_{\lambda\sigma}^P \varphi_P \right)_m := \int d\mathbf{r} d\mathbf{r}' \left[ \phi_\mu(\mathbf{r})\phi_\nu(\mathbf{r}) - \sum_P B_{\mu\nu}^P \varphi_P(\mathbf{r}) \right] m(\mathbf{r}, \mathbf{r}') \left[ \phi_\lambda(\mathbf{r}')\phi_\sigma(\mathbf{r}') - \sum_P B_{\lambda\sigma}^P \varphi_P(\mathbf{r}') \right] \quad (\text{S25})$$

$$= (\phi_\mu\phi_\nu|\phi_\lambda\phi_\sigma)_m - 2 \sum_P B_{\mu\nu}^P (\phi_\mu\phi_\nu|\varphi_P)_m + \sum_{PQ} B_{\mu\nu}^P B_{\lambda\sigma}^Q M_{PQ}. \quad (\text{S26})$$

The two- and three center integrals appearing in Eq. (S26) are defined as

$$(\phi_\mu\phi_\nu|\varphi_P)_m \equiv (\varphi_P|\phi_\mu\phi_\nu)_m = \int d\mathbf{r} d\mathbf{r}' \phi_\mu(\mathbf{r})\phi_\nu(\mathbf{r}) m(\mathbf{r}, \mathbf{r}') \varphi_P(\mathbf{r}'), \quad (\text{S27})$$

$$M_{PQ} \equiv (\varphi_P|\varphi_Q)_m = \int d\mathbf{r} d\mathbf{r}' \varphi_P(\mathbf{r}) m(\mathbf{r}, \mathbf{r}') \varphi_Q(\mathbf{r}'). \quad (\text{S28})$$

Differentiating Eq. (S26) with respect to  $B_{\mu\nu}^P$  and setting the result to zero leads to the RI expansion coefficients,<sup>34</sup>

$$B_{\mu\nu}^P = \sum_Q (\mathbf{M}^{-1})_{PQ} (\phi_\mu\phi_\nu|\varphi_Q)_m. \quad (\text{S29})$$

$\mathbf{M}^{-1}$  is the inverse of matrix  $\mathbf{M}$  that is defined in Eq. (S28). Inserting Eq. (S29) into Eqs. (S24)/(S23), one obtains the equation that is used to replace four-center Coulomb integrals by two-center and three-center integrals,

$$(\phi_\mu\phi_\nu|\phi_\lambda\phi_\sigma) = \sum_{PQRT} (\phi_\mu\phi_\nu|\varphi_P)_m (\mathbf{M}^{-1})_{PQ} V_{QR} (\mathbf{M}^{-1})_{RT} (\varphi_T|\phi_\lambda\phi_\sigma)_m, \quad (\text{S30})$$

where the two-center Coulomb matrix is

$$V_{PQ} = \int d\mathbf{r} d\mathbf{r}' \varphi_P(\mathbf{r}) \frac{1}{|\mathbf{r} - \mathbf{r}'|} \varphi_Q(\mathbf{r}'). \quad (\text{S31})$$

In practical calculations, the RI basis  $\{\varphi_P\}$  is large. This leads to linear dependencies in the RI basis which results in large inverse matrix elements  $M_{PQ}^{-1}$  and thus large expansion coefficients  $B_{\mu\nu}^P$ . In this work, we regularize Eq. (S25)/(S26), i.e. we minimize

$$\left( \phi_\mu\phi_\nu - \sum_P B_{\mu\nu}^P \varphi_P \middle| \phi_\lambda\phi_\sigma - \sum_P B_{\lambda\sigma}^P \varphi_P \right)_m + \alpha^2 \sum_P (B_{\mu\nu}^P)^2, \quad (\text{S32})$$

where  $\alpha \geq 0$ . Differentiating Eq. (S32) with respect to  $B_{\mu\nu}^P$  and setting the result to zero leads to

$$B_{\mu\nu}^P = \sum_Q \left( (\mathbf{M} + \alpha \mathbf{1})^{-1} \right)_{PQ} (\phi_\mu\phi_\nu|\varphi_Q)_m, \quad (\text{S33})$$

where  $\mathbf{1}$  is the identity matrix.

In the algorithm described in the manuscript, we incorporate the regularized RI (S33), by inverting the matrix  $\mathbf{M}(\mathbf{k}) + \alpha \mathbf{1}$  to calculate the matrix denoted as  $\mathbf{M}^{-1}(\mathbf{k})$ ,

$$\mathbf{M}^{-1}(\mathbf{k}) := (\mathbf{M}(\mathbf{k}) + \alpha \mathbf{1})^{-1}. \quad (\text{S34})$$

We chose  $\alpha = 10^{-2}$  for all calculations in the manuscript. In Fig. S1, we show that the  $G_0W_0$  band gap of  $\text{MoS}_2$  converges relatively fast with the supercell size when choosing  $\alpha = 10^{-2}$  (blue traces) compared to  $\alpha = 10^{-3}$  (green traces) and to standard RI ( $\alpha = 0$ , brown traces). An even larger regularization  $\alpha = 10^{-1}$  hampers the RI expansion (S33); we observe that the  $G_0W_0$ @LDA band gap deviates by 0.03 eV for large cells compared to the  $G_0W_0$ @LDA band gap computed with smaller regularization parameters  $\alpha$ .

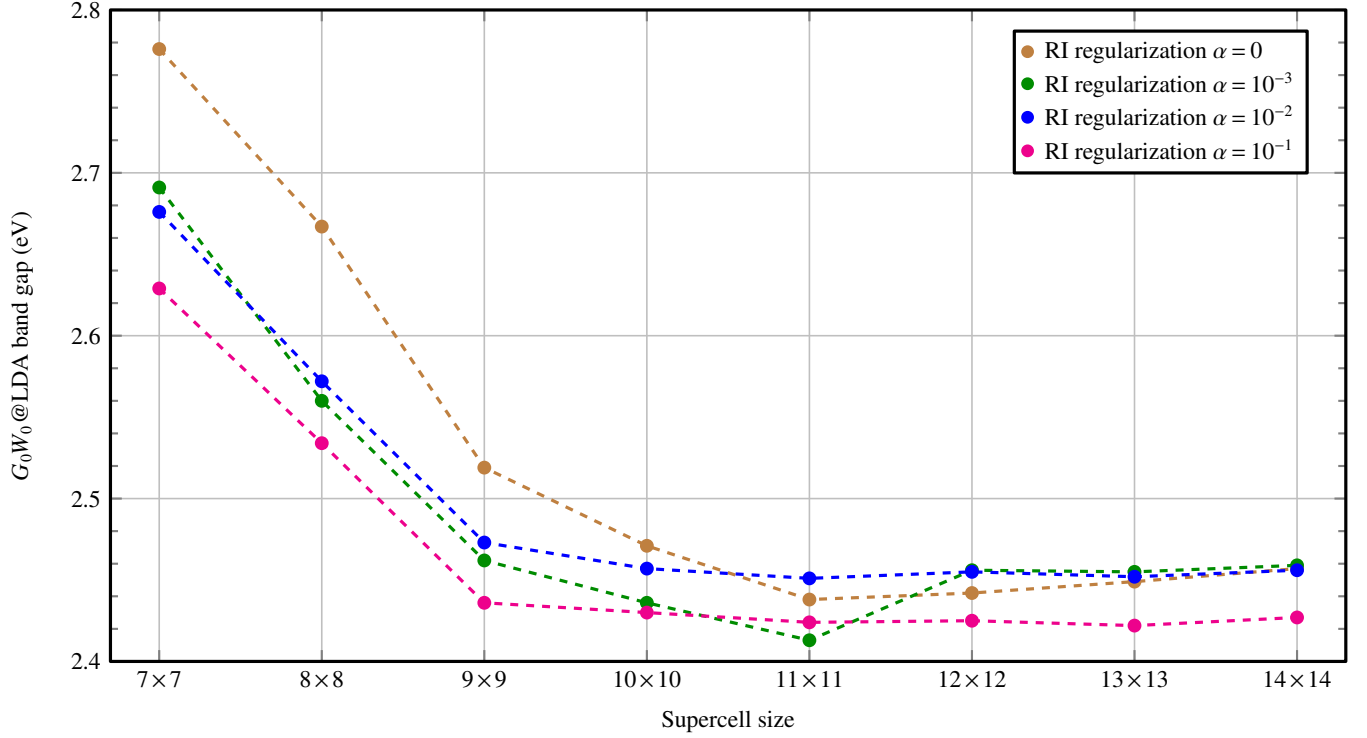

FIG. S1.  $G_0W_0$ @LDA gap for  $\text{MoS}_2$  as function of the supercell size for three values of the RI regularization parameter  $\alpha \in \{0, 10^{-3}, 10^{-2}, 10^{-1}\}$  [ $\alpha$  enters the  $GW$  algorithm via Eq. (S34)].

#### S4. CONVERGENCE WITH THE BASIS SET SIZE

We investigate how the  $G_0W_0$ @PBE bandgap of monolayer  $\text{MoS}_2$ ,  $\text{MoSe}_2$ ,  $\text{WS}_2$  and  $\text{WSe}_2$  converges with the basis set  $\{\phi_v\}$  for Bloch states and the auxiliary basis set  $\{\varphi_P\}$  from the resolution of the identity (RI), see Table S1. We also change the supercell size and the number of time and frequency points<sup>4</sup>. For Table I in the manuscript, we report the bold  $G_0W_0$ @PBE bandgap ( $10 \times 10$  supercell, 30 time/frequency points, TZV2P-MOLOPT basis set). Further investigating and improving the numerical convergence with the basis set size, supercell size and the time/frequency grid, will be subject of future work.

TABLE S1.  $G_0W_0$ @PBE bandgap of a monolayer  $\text{MoS}_2$ ,  $\text{MoSe}_2$ ,  $\text{WS}_2$ , and  $\text{WSe}_2$  for various different numerical parameters. We abbreviate "RI standard" for a standard RI basis set (example: 159 RI basis functions per  $\text{MoS}_2$  unit), "RI big" (225 RI basis functions per  $\text{MoS}_2$  unit) and "RI huge" (316 RI basis functions per  $\text{MoS}_2$  unit). The TZVP-MOLOPT and the TZV2P-MOLOPT basis sets are standard basis sets<sup>15,35</sup> used together with Goedecker-Teter-Hutter pseudopotentials<sup>17</sup>. As an example, the TZVP-MOLOPT-GTH basis set contains 35 Gaussians per Mo atom ( $4 \times s$ ,  $3 \times p$ ,  $3 \times d$ ,  $1 \times f$  functions) and 17 Gaussians per S atom ( $3 \times s$ ,  $3 \times p$ ,  $1 \times d$  functions). Inputs and outputs are available on github<sup>19</sup>.

|                 | Supercell      | Time/freq. grid points | Gaussian basis: TZVP-MOLOPT <sup>15,35</sup> |        |         | Gaussian basis: TZV2P-MOLOPT <sup>15,35</sup> |        |         |
|-----------------|----------------|------------------------|----------------------------------------------|--------|---------|-----------------------------------------------|--------|---------|
|                 |                |                        | RI standard                                  | RI big | RI huge | RI standard                                   | RI big | RI huge |
| $\text{MoS}_2$  | $10 \times 10$ | 10                     | 2.459                                        | 2.538  | 2.510   | 2.455                                         | 2.560  | 2.511   |
|                 | $11 \times 11$ | 10                     | 2.451                                        | 2.483  |         | 2.446                                         | 2.493  |         |
|                 | $12 \times 12$ | 10                     | 2.456                                        | 2.462  |         | 2.451                                         |        |         |
|                 | $10 \times 10$ | 20                     | 2.493                                        |        |         | 2.476                                         |        |         |
|                 | $10 \times 10$ | 30                     | 2.486                                        |        |         | <b>2.471</b>                                  |        |         |
| $\text{MoSe}_2$ | $10 \times 10$ | 10                     | 2.045                                        | 2.029  | 2.047   | 2.053                                         | 2.043  | 2.054   |
|                 | $11 \times 11$ | 10                     | 2.047                                        | 2.051  |         | 2.054                                         | 2.058  |         |
|                 | $10 \times 10$ | 20                     | 2.079                                        |        |         | 2.074                                         |        |         |
|                 | $10 \times 10$ | 30                     | 2.077                                        |        |         | <b>2.071</b>                                  |        |         |
| $\text{WS}_2$   | $10 \times 10$ | 10                     | 2.796                                        | 2.786  | 2.787   | 2.793                                         | 2.782  | 2.771   |
|                 | $11 \times 11$ | 10                     | 2.798                                        | 2.786  |         | 2.788                                         | 2.784  |         |
|                 | $10 \times 10$ | 20                     | 2.800                                        |        |         | 2.814                                         |        |         |
|                 | $10 \times 10$ | 30                     | 2.814                                        |        |         | <b>2.812</b>                                  |        |         |
| $\text{WSe}_2$  | $10 \times 10$ | 10                     | 2.365                                        | 2.350  | 2.355   | 2.347                                         | 2.333  | 2.336   |
|                 | $11 \times 11$ | 10                     | 2.368                                        | 2.354  |         | 2.344                                         | 2.338  |         |
|                 | $10 \times 10$ | 20                     | 2.381                                        |        |         | 2.362                                         |        |         |
|                 | $10 \times 10$ | 30                     | 2.378                                        |        |         | <b>2.367</b>                                  |        |         |

## S5. ADDITIONAL CONVERGENCE CHECKS

In Fig. S2, we present additional convergence checks of the  $GW$  bandgap with the minimax time/frequency grid size, the  $k$ -point mesh size, the filter parameter of sparse tensor operations, and with the box height.

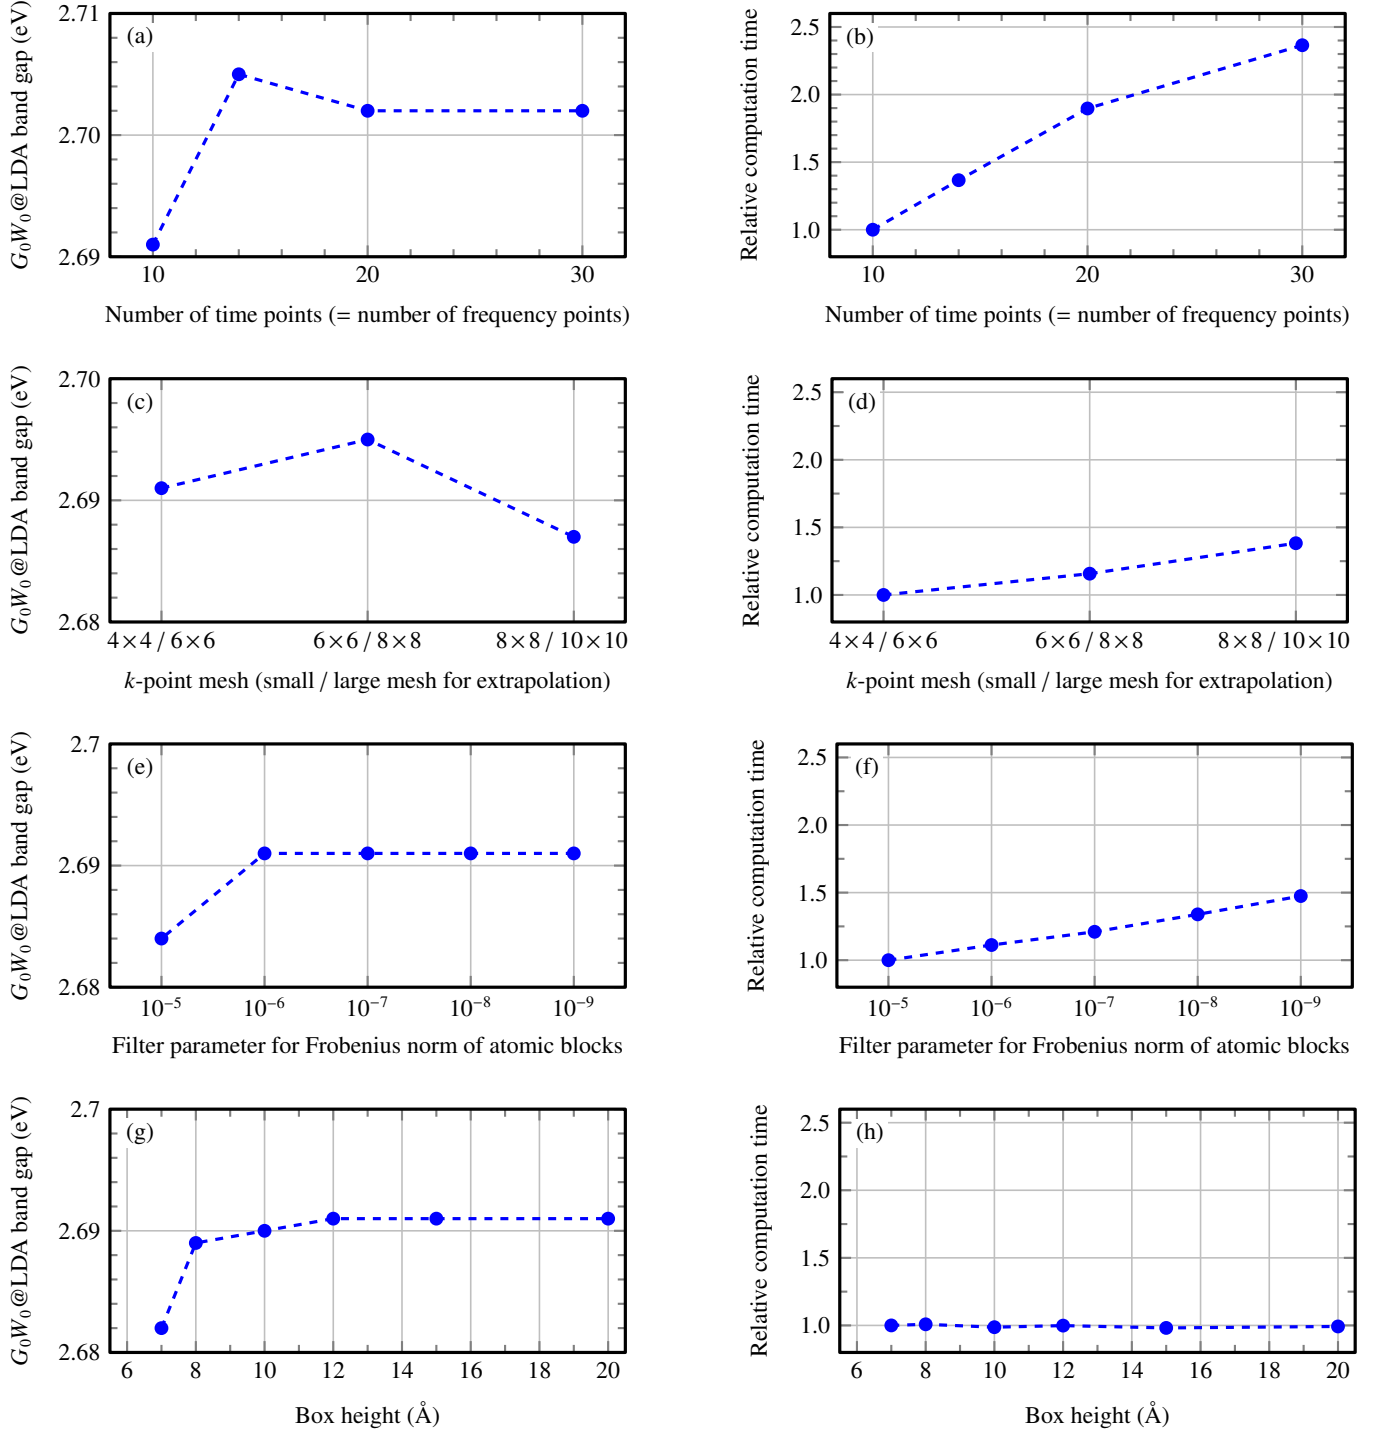

FIG. S2. Convergence tests of the low-scaling  $GW$  algorithm for a  $7 \times 7$  supercell of  $\text{MoS}_2$ . We benchmark the convergence of the  $G_0W_0$  gap as function of the following convergence parameters: (a)/(b) number of time/frequency points, (c)/(d)  $k$ -point mesh size, (e)/(f) filter parameter of sparse tensor operations and (g)/(h) box height. Shown are the bandgap (left column) and the computation time (right column). Standard settings in the manuscript are 10 time/frequency points, a  $4 \times 4 / 6 \times 6$   $k$ -point mesh, a filter  $10^{-6}$  and 15  $\text{\AA}$  box height.

## S6. CUTOFF RADIUS OF THE TRUNCATED COULOMB METRIC FOR THE RESOLUTION OF THE IDENTITY

The choice of the RI metric  $m(\mathbf{r}, \mathbf{r}')$  is crucial for making the low-scaling  $GW$  algorithm from the manuscript efficient. One possibility is the overlap metric<sup>3,4,34</sup>,

$$m(\mathbf{r}, \mathbf{r}') = \delta(\mathbf{r} - \mathbf{r}') \quad (\text{S35})$$

where  $\delta$  is the Dirac distribution. The overlap metric is space-local in the sense that the auxiliary Gaussian basis functions  $\varphi_P$  do not overlap with atomic-orbital basis function products  $\phi_\mu\phi_\nu$  in Eq. (S27) if there is enough distance between their centers. This leads to vanishing three-center overlap matrix elements  $(\mu\nu|P)_m$  and increasing computational efficiency due to sparsity.

In contrast, the Coulomb metric

$$m_C(\mathbf{r}, \mathbf{r}') = \frac{1}{|\mathbf{r} - \mathbf{r}'|} \quad (\text{S36})$$

couple RI basis functions  $\varphi_P$  and Gaussians basis function pairs  $\phi_\mu\phi_\nu$  in Eq. (S27) over effectively infinite distances due to the slow polynomial decay of  $1/|\mathbf{r} - \mathbf{r}'|$ . With the Coulomb metric, no sparsity can be gained hampering its usage in low-scaling  $GW$  algorithms. In standard  $O(N^4)$  algorithms, each Gaussian  $\phi_\mu, \phi_\nu$  is transformed to the delocalized molecular orbital basis  $\{\psi_n\}$  losing all sparsity anyway<sup>9</sup>. In such a conventional algorithm, where sparsity cannot be exploited, the Coulomb metric is the optimal choice because the RI factorization given in Eq. (S30) converges very quickly with respect to the RI basis set size.<sup>34</sup> The Coulomb metric thus yields generally higher accuracy than the overlap metric.

In this work, we employ the truncated Coulomb metric<sup>4-6</sup>

$$m_{r_c}(\mathbf{r}, \mathbf{r}') = \begin{cases} \frac{1}{|\mathbf{r} - \mathbf{r}'|} & \text{if } |\mathbf{r} - \mathbf{r}'| < r_c, \\ 0 & \text{else,} \end{cases} \quad (\text{S37})$$

where the Coulomb interaction is cut after a distance  $r_c$ . In the limit of a large cutoff radius  $r_c$ , the truncated Coulomb metric turns into the Coulomb metric,  $\lim_{r_c \rightarrow \infty} m_{r_c}(\mathbf{r}, \mathbf{r}') = 1/|\mathbf{r} - \mathbf{r}'|$ . For a small cutoff radius  $r_c$ , calculations based on the truncated Coulomb metric are equivalent to calculations based on the overlap metric. The truncated Coulomb metric combines the attractive features of the Coulomb metric and the overlap metric: high accuracy due to the near-sighted Coulomb operator and preservation of sparsity due to the locality of  $m_{r_c}(\mathbf{r}, \mathbf{r}')$ . The RI factorization in Eq. (S30) is exact in the limit of a complete RI basis, independent of the chosen RI metric. Therefore, truncating the Coulomb operator with a finite  $r_c$  does not affect the accuracy of the  $GW$  algorithm as long as the RI basis is sufficiently large.

We show the convergence of the  $G_0W_0$  bandgap of  $\text{MoS}_2$  with the RI basis set size  $\{\varphi_P(\mathbf{r})\}$  in Fig. S3. It is seen that the convergence with the RI basis is fast when using a cutoff radius  $r_c = 3 \text{ \AA}$ , and the convergence is slower for  $r_c = 2 \text{ \AA}$ . For a large RI basis set with 240 auxiliary functions per  $\text{MoS}_2$  unit, we find that the bandgap for  $r_c = 2 \text{ \AA}$  matches the bandgap for  $r_c = 3 \text{ \AA}$  within 0.02 eV. Overall, we confirm that  $r_c = 3 \text{ \AA}$  is a good choice.

We note that in plane-wave implementations, RI with different metrics is not discussed. The reason is that the Coulomb matrix, the truncated Coulomb matrix and the overlap matrix are diagonal in the plane-wave basis. As consequence, RI factorizations as in Eq. (S30) are identical for the three different metrics when using plane wave basis functions. More details can be found in the Supporting Information of Ref. 4.

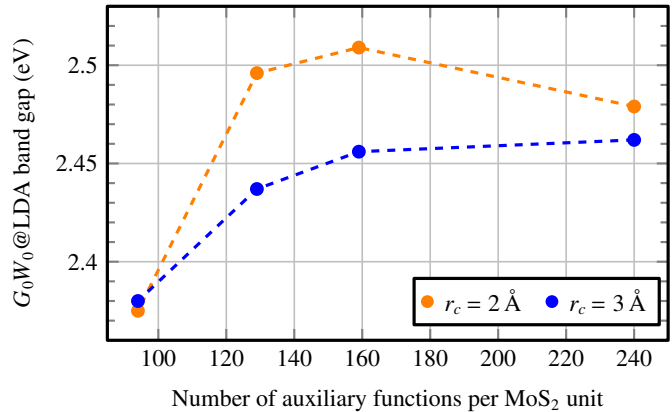

FIG. S3. Gap of monolayer  $\text{MoS}_2$  ( $12 \times 12$  supercell) as function of the number of auxiliary functions  $\{\varphi_P\}$  and the cutoff radius in RI metric.

## S7. COMPARISON OF THE LOW-SCALING GW ALGORITHM TO A STANDARD-SCALING GW ALGORITHM

In Fig. S4, we compare the periodic, Gaussian-based, low-scaling GW algorithm from the manuscript with a periodic, Gaussian-based GW algorithm that operates in frequency only and avoids sparse matrix-tensor operations.

| Periodic GW algorithm in a Gaussian basis with RI<br>(similar to the algorithm by Zhu and Chan <sup>9</sup> )                                                                                                                                                                                                                                                                                                                                                                                                                                                                                                                                  | Low-scaling periodic GW algorithm in a Gaussian basis with RI<br>(this work)                                                                                                                                                                                                                                                                                                                                                                                                                                                                                                                                                                                                                                                                                                                                                                                                                                                                                                                                                                                                                                        |
|------------------------------------------------------------------------------------------------------------------------------------------------------------------------------------------------------------------------------------------------------------------------------------------------------------------------------------------------------------------------------------------------------------------------------------------------------------------------------------------------------------------------------------------------------------------------------------------------------------------------------------------------|---------------------------------------------------------------------------------------------------------------------------------------------------------------------------------------------------------------------------------------------------------------------------------------------------------------------------------------------------------------------------------------------------------------------------------------------------------------------------------------------------------------------------------------------------------------------------------------------------------------------------------------------------------------------------------------------------------------------------------------------------------------------------------------------------------------------------------------------------------------------------------------------------------------------------------------------------------------------------------------------------------------------------------------------------------------------------------------------------------------------|
| <p>Irreducible polarizability (scaling: <math>N_k^2 N_{\text{occ}} N_{\text{virt}} N_{\text{RI}}^2</math>)</p> $\chi_{PQ}(\mathbf{k}, i\omega) = \frac{1}{N_k} \sum_{ia\mathbf{q}} (i\mathbf{k} a\mathbf{k}-\mathbf{q}   P\mathbf{q}) \frac{2(\varepsilon_{i\mathbf{k}} - \varepsilon_{a\mathbf{k}-\mathbf{q}})}{\omega^2 + (\varepsilon_{i\mathbf{k}} - \varepsilon_{a\mathbf{k}-\mathbf{q}})^2} (i\mathbf{k} a\mathbf{k}-\mathbf{q}   Q\mathbf{q})$ <p><math>(i\mathbf{k} a\mathbf{k}-\mathbf{q}   P\mathbf{q})</math> are three-center integrals of the RI metric <math>m(\mathbf{r}, \mathbf{r}')</math>, see Ref. 9 for a definition.</p> | <p>Irreducible polarizability</p> <ol style="list-style-type: none"> <li>1. <math>\Gamma</math>-point only (Eq. (S4), scaling for large systems<sup>4</sup>: <math>N^2</math>): <math display="block">\chi_{PQ}(\mathbf{0}, i\tau) = \sum_{\lambda\nu\mu\sigma} (\mu\mathbf{0} \nu\mathbf{0}   P\mathbf{0}) G_{\mu\lambda}(\mathbf{0}, -i\tau) (\lambda\mathbf{0} \sigma\mathbf{0}   Q\mathbf{0}) G_{\nu\sigma}(\mathbf{0}, i\tau)</math> </li> <li>2. <math>\Gamma</math>-point to arbitrary <math>k</math>-point [Eq. (S8), (S9)]: <math display="block">\chi_{PQ}(\mathbf{k}, i\tau) = \sum_{\mathbf{R}} e^{i\mathbf{k}\cdot\mathbf{R}} \cdot \begin{cases} \chi_{PQ}(\mathbf{0}, i\tau) &amp; \text{if } \varphi_P^{\mathbf{0}}, \varphi_Q^{\mathbf{R}} \text{ closest,} \\ 0 &amp; \text{else} \end{cases}</math> </li> <li>3. Time to frequency transform [Eq. (S10)]: <math display="block">\chi_{PQ}(\mathbf{k}, i\omega) = \int d\tau \cos(\omega\tau) \chi_{PQ}(\mathbf{k}, i\tau)</math> </li> <li>4. Remove all spurious negative eigenvalues of <math>\chi_{PQ}(\mathbf{k}, i\omega)</math></li> </ol> |
| <p>Dielectric function (Eq. (10) in manuscript, scaling: <math>N_k N_{\text{RI}}^3</math>)</p> $\epsilon(\mathbf{k}, i\omega) = \mathbf{1} - \mathbf{V}^{0.5}(\mathbf{k}) \mathbf{M}^{-1}(\mathbf{k}) \chi(\mathbf{k}, i\omega) \mathbf{M}^{-1}(\mathbf{k}) \mathbf{V}^{0.5}(\mathbf{k})$                                                                                                                                                                                                                                                                                                                                                      | <p>Dielectric function (Eq. (S11), scaling: <math>N_k N_{\text{RI}}^3</math>)</p> $\epsilon(\mathbf{k}, i\omega) = \mathbf{1} - \mathbf{V}^{0.5}(\mathbf{k}) \mathbf{M}^{-1}(\mathbf{k}) \chi(\mathbf{k}, i\omega) \mathbf{M}^{-1}(\mathbf{k}) \mathbf{V}^{0.5}(\mathbf{k})$                                                                                                                                                                                                                                                                                                                                                                                                                                                                                                                                                                                                                                                                                                                                                                                                                                        |
| <p>Screened Coulomb potential<br/>(Eqs. (13), (17) in manuscript, scaling: <math>N_k N_{\text{RI}}^3</math>)</p> $\mathbf{W}(\mathbf{k}, i\omega) = \mathbf{V}_{\text{rc}}(\mathbf{k}) + \mathbf{V}^{0.5}(\mathbf{k}) (\epsilon^{-1}(\mathbf{k}, i\omega) - \mathbf{Id}) \mathbf{V}^{0.5}(\mathbf{k})$ $\tilde{\mathbf{W}}(\mathbf{k}, i\omega) = \mathbf{M}^{-1}(\mathbf{k}) \mathbf{W}(\mathbf{k}, i\omega) \mathbf{M}^{-1}(\mathbf{k})$                                                                                                                                                                                                     | <p>Screened Coulomb potential<br/>(Eqs. (S14) - (S18) in manuscript, scaling: <math>N_k N_{\text{RI}}^3</math>)</p> $\mathbf{W}(\mathbf{k}, i\omega) = \mathbf{V}_{\text{rc}}(\mathbf{k}) + \mathbf{V}^{0.5}(\mathbf{k}) (\epsilon^{-1}(\mathbf{k}, i\omega) - \mathbf{Id}) \mathbf{V}^{0.5}(\mathbf{k})$ $\mathbf{W}^{\mathbf{R}}(i\omega) = \frac{1}{N_k} \sum_{\mathbf{k}} e^{i\mathbf{k}\cdot\mathbf{R}} \mathbf{W}(\mathbf{k}, i\omega)$ $W_{PQ}^{\text{MIC}}(i\omega) = W_{PQ}^{\mathbf{R}^{\min}}(i\omega), \quad \mathbf{R}^{\min} = \underset{\mathbf{R}}{\text{argmin}}  \mathbf{R}_P - (\mathbf{R}_Q + \mathbf{R}) $ $\tilde{\mathbf{W}}(i\omega) = \mathbf{M}^{-1}(\mathbf{0}) \mathbf{W}^{\text{MIC}}(i\omega) \mathbf{M}^{-1}(\mathbf{0})$                                                                                                                                                                                                                                                                                                                                                            |
| <p>Self-energy (scaling: <math>N_k^2 N_{\text{AO}}^2 N_{\text{RI}}^2</math>)</p> $\Sigma_{n\mathbf{k}}(i\omega) = -\frac{1}{2\pi N_k} \sum_{m\mathbf{q}} \int d\omega' \frac{1}{i(\omega - \omega') + \varepsilon_{\text{F}} - \varepsilon_{m\mathbf{k}-\mathbf{q}}} \times \sum_{PQ} (n\mathbf{k} m\mathbf{k}-\mathbf{q}   P\mathbf{q}) \tilde{W}_{PQ}(\mathbf{q}, i\omega') (n\mathbf{k} m\mathbf{k}-\mathbf{q}   Q\mathbf{q})$                                                                                                                                                                                                              | <p>Self-energy</p> <ol style="list-style-type: none"> <li>1. <math>\Gamma</math>-point only (Eq. (S19), scaling for large systems<sup>4</sup>: <math>N^2</math>) <math display="block">\Sigma_{\lambda\sigma}(\mathbf{0}, i\tau) = i \sum_{\nu\mu PQ} (\lambda\mathbf{0} \mu\mathbf{0}   Q\mathbf{0}) G_{\mu\nu}(\mathbf{0}, i\tau) (\nu\mathbf{0} \sigma\mathbf{0}   P\mathbf{0}) \tilde{W}_{PQ}(i\tau)</math> </li> <li>2. Transformation to Bloch states (Eq. (S20), (S21) scaling: <math>N_k N_{\text{AO}}^3</math>) <math display="block">\Sigma_{\lambda\sigma}(\mathbf{k}, i\tau) = \sum_{\mathbf{R}} e^{i\mathbf{k}\cdot\mathbf{R}} \cdot \begin{cases} \Sigma_{\lambda\sigma}(\mathbf{0}, i\tau) &amp; \text{if } \phi_{\lambda}^{\mathbf{0}}, \phi_{\sigma}^{\mathbf{R}} \text{ closest,} \\ 0 &amp; \text{else} \end{cases}</math> <math display="block">\Sigma_{n\mathbf{k}}(i\tau) = \sum_{\lambda\sigma} C_{n\lambda}^*(\mathbf{k}) \Sigma_{\lambda\sigma}(\mathbf{k}, i\tau) C_{n\sigma}(\mathbf{k})</math> </li> </ol>                                                                              |

FIG. S4. Left column: Periodic GW algorithm with Gaussian basis functions, similar to Ref. 9. Right column: Periodic GW algorithm with Gaussian basis functions from this work. Mathematical symbols are defined in Sec. S1.

## S8. REQUIRED NUMBER OF FLOATING POINT OPERATIONS OF A PLANE-WAVE BASED GW ALGORITHM

The computational effort of applying plane-wave based *GW* algorithms to two-dimensional materials is large. The computational bottleneck is computing the irreducible polarizability,

$$\chi_{\mathbf{G}\mathbf{G}'}(\mathbf{q}, i\omega) = \sum_n^{\text{occ}} \sum_{n'}^{\text{empty}} \sum_{\mathbf{k}} \frac{\langle n\mathbf{k}+\mathbf{q} | e^{i(\mathbf{q}+\mathbf{G})\cdot\mathbf{r}} | n'\mathbf{k} \rangle \langle n'\mathbf{k} | e^{-i(\mathbf{q}+\mathbf{G}')\cdot\mathbf{r}} | n\mathbf{k}+\mathbf{q} \rangle}{\varepsilon_{n\mathbf{k}+\mathbf{q}} - \varepsilon_{n'\mathbf{k}} + i\omega}, \quad N_{\text{flop}}^{\text{PW}} = 4N_{\mathbf{q}}N_{\omega}N_{\mathbf{G}}^2N_{\text{occ}}N_{\text{empty}}N_{\mathbf{k}}, \quad (\text{S38})$$

where  $\mathbf{G}, \mathbf{G}'$  are reciprocal lattice vectors,  $\mathbf{q}$  is a vector in the first Brillouin zone,  $n, n'$  refer to occupied and empty bands, respectively, and the brackets in the second line denote integrals of a plane wave and Bloch states.  $N_{\text{flop}}^{\text{PW}}$  in Eq. (S38) denotes the number of floating point operations (real double precision) which is the product of:

- a factor 4 to account for the complex numbers,
- the number of  $\mathbf{q}$ -points,  $N_{\mathbf{q}}$ , to discretize  $\chi(\mathbf{q})$  in the Brillouin zone, (a  $3 \times 3$  mesh has been chosen in Ref. 36 for a large-scale calculation on a 2D material; considering time-reversal symmetry  $\mathbf{q} \leftrightarrow -\mathbf{q}$ , a  $3 \times 3$  mesh contains 5 independent  $\mathbf{q}$ -points; the  $3 \times 3$  mesh is necessary to resolve the divergence of the Coulomb interaction at  $\mathbf{q} \rightarrow \mathbf{0}$ )
- the number of frequency points,  $N_{\omega}$ , (We assume full-frequency calculations<sup>37</sup> with  $N_{\omega} = 10$  as in the main manuscript. When using a plasmon-pole model<sup>36,37</sup>, one would have  $N_{\omega} = 1$ .)
- the number of plane waves,  $N_{\mathbf{G}}^2$ , where the square is due to the row and column index of  $\chi$ , (From the energy cutoff  $E_c = 25 \text{ Ry}$ <sup>36,37</sup>, we estimate the plane-wave cutoff  $G_c = \sqrt{2m_e E_c}/\hbar$  and the corresponding reciprocal sphere volume  $\Omega_c = 4\pi G_c^3/3$ . From the  $1 \times 1$  supercell size  $V_{\text{cell}} = 2.5 \text{ \AA} \times 2.5 \text{ \AA} \times 25 \text{ \AA}$  of a 2D semiconductor, we estimate the Brillouin zone volume  $\Omega_{\text{BZ}} = (2\pi)^3/V_{\text{cell}}$  which leads to  $N_{\mathbf{G}} = \Omega_c/\Omega_{\text{BZ}} = 2200$  for a  $1 \times 1$  supercell.)
- the number of occupied bands,  $N_{\text{occ}}$ , (which follows from the employed pseudopotential)
- the number of empty bands,  $N_{\text{empty}}$ , (which is a convergence parameter and has been chosen in Ref. 37 as 6000 for a  $1 \times 1$  cell, we assume a factor 10 less empty bands for large-scale calculations) and
- the number of  $\mathbf{k}$ -points,  $N_{\mathbf{k}}$ , for the Brillouin zone sum  $\sum_{\mathbf{k}}$  (for large-scale calculations, the  $\Gamma$ -point is sufficient, i.e.  $N_{\mathbf{k}} = 1$ ).

We estimate the required floating point operations to evaluate Eq. (S38) in Table S2.

TABLE S2. We estimate the required operations to compute the irreducible polarizability in a plane-wave basis set, Eq. (S38), for a 2D semiconductor as monolayer MoS<sub>2</sub>. Computational parameters are chosen similar to Refs. 36 and 37.

| Supercell | $N_{\text{occ}}$ | $N_{\text{empty}}$ | $N_{\mathbf{G}}$ | $N_{\mathbf{q}}$ | $N_{\mathbf{k}}$ | $N_{\omega}$ | $N_{\text{flop}}^{\text{PW}}$ |
|-----------|------------------|--------------------|------------------|------------------|------------------|--------------|-------------------------------|
| 1x1       | 13               | 600                | 2200             | 20               | 10               | 10           | $3.0 \cdot 10^{14}$           |
| 2x2       | 52               | 2400               | 8800             | 5                | 3                | 10           | $5.8 \cdot 10^{15}$           |
| 3x3       | 117              | 5400               | 19800            | 5                | 2                | 10           | $9.9 \cdot 10^{16}$           |
| 4x4       | 208              | 9600               | 35200            | 5                | 1                | 10           | $4.9 \cdot 10^{17}$           |
| 5x5       | 325              | 15000              | 55000            | 5                | 1                | 10           | $2.9 \cdot 10^{18}$           |
| 6x6       | 468              | 21600              | 79200            | 5                | 1                | 10           | $1.3 \cdot 10^{19}$           |
| 7x7       | 637              | 29400              | 107800           | 5                | 1                | 10           | $4.4 \cdot 10^{19}$           |
| 8x8       | 832              | 38400              | 140800           | 5                | 1                | 10           | $1.3 \cdot 10^{20}$           |
| 9x9       | 1053             | 48600              | 178200           | 5                | 1                | 10           | $3.3 \cdot 10^{20}$           |
| 10x10     | 1300             | 60000              | 220000           | 5                | 1                | 10           | $7.6 \cdot 10^{20}$           |
| 11x11     | 1573             | 72600              | 266200           | 5                | 1                | 10           | $1.6 \cdot 10^{21}$           |
| 12x12     | 1872             | 86400              | 316800           | 5                | 1                | 10           | $3.2 \cdot 10^{21}$           |
| 13x13     | 2197             | 101400             | 371800           | 5                | 1                | 10           | $6.2 \cdot 10^{21}$           |
| 14x14     | 2548             | 117600             | 431200           | 5                | 1                | 10           | $1.1 \cdot 10^{22}$           |

## S9. REQUIRED NUMBER OF FLOATING POINT OPERATIONS OF THE GW ALGORITHM FROM THIS WORK

The computation of  $\chi$  in the  $G_0W_0$  algorithm from this work is given in Eq. (S4). We execute Eq. (S4) in three steps<sup>4</sup>,

$$\chi_{PQ}(\mathbf{q}=\mathbf{0}, i\tau) = \sum_{\lambda\nu} X_{\lambda\nu P}(i\tau) Y_{\lambda\nu Q}(i\tau), \quad N_{\text{flop}} = N_\tau N_{\text{RI}}^2 N_{\text{AO}}^2 \alpha, \quad (\text{S39})$$

$$X_{\lambda\nu P}(i\tau) = \sum_{\mu} (\mu\nu|P) G_{\mu\lambda}(\mathbf{k}=\mathbf{0}, -i\tau), \quad Y_{\lambda\nu Q}(i\tau) = \sum_{\sigma} (\lambda\sigma|Q) G_{\nu\sigma}(\mathbf{k}=\mathbf{0}, i\tau), \quad N_{\text{flop}} = 2N_\tau N_{\text{RI}} N_{\text{AO}}^3 \alpha. \quad (\text{S40})$$

The required floating point operations,  $N_{\text{flop}}$ , is computed as a product of:

- the number of time points,  $N_\tau$ , [cf. Fig. S2 (a)]
- the number of auxiliary RI basis functions,  $N_{\text{RI}}$ ,
- the number of Gaussian basis functions  $N_{\text{AO}}$  to expand Bloch states,
- $\alpha$  is the percentage of matrix elements  $(\mu\nu|P)$  above a certain filter threshold [cf. Fig. S2 (c)]. All matrix elements smaller than the threshold are neglected in the computation. For a large number of atoms  $N_{\text{at}}$  in the unit cell,  $\alpha$  is smaller than one,

$$\alpha \sim \left( \frac{N_{\text{at}}^*}{N_{\text{at}}} \right)^2, \quad (\text{S41})$$

where  $N_{\text{at}}^*$  is the number of atoms of the largest system without sparsity, i.e.  $\alpha = 1$  for a system with  $N_{\text{at}}^*$  atoms. With Eq. (S41), the computational scaling of Eqs. (S39) and (S40) is  $O(N_{\text{at}}^2)$  for  $N_{\text{at}} > N_{\text{at}}^*$ .

The number of auxiliary Gaussians is typically two to three times larger than the basis set for Bloch orbitals,  $N_{\text{RI}} \approx 2\text{-}3 \cdot N_{\text{AO}}$ . This results in a similar number of floating point operations of Eq. (S39) and (S40). Eq. (S19) for the self-energy is expected to require a similar number of floating point operations as Eq. (S39) and (S40). The complex diagonalization of  $\chi_{PQ}(\mathbf{k}, i\omega)$  to remove spurious negative eigenvalues [described after Eq. (S10)] is estimated to require  $10N_{\text{RI}}^3 N_{\mathbf{k}} N_\omega$  operations, where  $N_\omega = N_\tau$ .<sup>4</sup> We choose a  $4 \times 4$  and  $6 \times 6$   $k$ -mesh to extrapolate the Brillouin zone integration in Eq. (S15). This extrapolation requires  $N_{\mathbf{k}} = 26$  kpoints when considering time-reversal symmetry  $\mathbf{k} \leftrightarrow -\mathbf{k}$ .

Summarizing, we estimate the total required number of floating point operations as

$$N_{\text{flop}}^{\text{Gauss}} = 4N_\tau N_{\text{RI}}^2 N_{\text{AO}}^2 \alpha + 10N_{\text{RI}}^3 N_{\mathbf{k}} N_\omega. \quad (\text{S42})$$

Results for  $N_{\text{flop}}^{\text{Gauss}}$  for monolayer 2D semiconductors are summarized in Table S3.

TABLE S3. Required number of operations (S42) to execute the  $G_0W_0$  algorithm from this work for a 2D semiconductor as monolayer MoS<sub>2</sub>.

| Supercell | $N_{\text{AO}}$ | $N_{\text{RI}}$ | $N_\tau = N_\omega$ | $\alpha$ | $N_{\mathbf{k}}$ | $N_{\text{flop}}^{\text{Gauss}}$ |
|-----------|-----------------|-----------------|---------------------|----------|------------------|----------------------------------|
| 1x1       | 69              | 159             |                     | 1.000    |                  |                                  |
| 9x9       | 5589            | 12879           | 10                  | 0.160    | 26               | $3.9 \cdot 10^{16}$              |
| 10x10     | 6900            | 15900           | 10                  | 0.105    | 26               | $6.1 \cdot 10^{16}$              |
| 11x11     | 8349            | 19239           | 10                  | 0.072    | 26               | $9.3 \cdot 10^{16}$              |
| 12x12     | 9936            | 22896           | 10                  | 0.051    | 26               | $1.4 \cdot 10^{17}$              |
| 13x13     | 11661           | 26871           | 10                  | 0.037    | 26               | $1.9 \cdot 10^{17}$              |
| 14x14     | 13524           | 31164           | 10                  | 0.027    | 26               | $2.7 \cdot 10^{17}$              |

## S10. FLOATING POINT OPERATIONS FOR THE LARGEST MOSE<sub>2</sub>/WS<sub>2</sub> HETEROSTRUCTURE WITH 984 ATOMS

We evaluate Eqs. (S38) and (S42) to compute the required number of floating point operations for the 984-atom MoSe<sub>2</sub>/WS<sub>2</sub> heterostructure shown in Fig. 4 in the manuscript. For the large-scale Gaussian-based algorithm from this work, we have the computational parameters (defined in Sec. S9) and corresponding operations  $N_{\text{flop}}^{\text{Gauss}}$  [Eq. (S42)]:

$$N_{\tau} = N_{\omega} = 10, \quad N_{\text{RI}} = 49441, \quad N_{\text{AO}} = 22632, \quad \alpha = 0.66\%, \quad N_{\mathbf{k}} = 26, \quad N_{\text{flop}}^{\text{Gauss}} = 6.5 \cdot 10^{17}. \quad (\text{S43})$$

For a plane-wave  $G_0W_0$  algorithm, the relevant computational parameters and corresponding operations  $N_{\text{flop}}^{\text{PW}}$  [Eq. (S38)] are

$$N_{\omega} = 10, \quad N_{\text{occ}} = 4264, \quad N_{\text{empty}} = 196800, \quad N_{\text{G}} = 320000, \quad N_{\mathbf{q}} = 5, \quad N_{\mathbf{k}} = 1, \quad N_{\text{flop}}^{\text{PW}} = 1.7 \cdot 10^{22}. \quad (\text{S44})$$

## S11. TIMINGS OF THE GW ALGORITHM

TABLE S4. Timings of  $G_0W_0$ @LDA calculations on monolayer MoSe<sub>2</sub> supercells of different size on Supermuc-NG (processor type: Intel Skylake Xeon Platinum 8174, 48 cores per node, 768 GB memory per node).

| Supercell size | Number of nodes | Total time (h) | Time of Eq. (S4) (h) | Time of diag. of $\chi_{PQ}(i\omega, \mathbf{k})$ (h) | Time of Eq. (S19) (h) |
|----------------|-----------------|----------------|----------------------|-------------------------------------------------------|-----------------------|
| 9 × 9          | 6               | 8.7            | 1.8                  | 1.5                                                   | 4.7                   |
| 10 × 10        | 12              | 7.1            | 1.3                  | 1.6                                                   | 3.6                   |
| 11 × 11        | 20              | 7.8            | 1.3                  | 2.4                                                   | 3.3                   |
| 12 × 12        | 22              | 10.0           | 1.5                  | 3.1                                                   | 4.3                   |
| 13 × 13        | 28              | 13.1           | 1.8                  | 4.9                                                   | 4.9                   |
| 14 × 14        | 34              | 15.5           | 1.9                  | 6.1                                                   | 5.5                   |

\* [jan.wilhelm@physik.uni-regensburg.de](mailto:jan.wilhelm@physik.uni-regensburg.de)

- <sup>1</sup> V. Blum, R. Gehrke, F. Hanke, P. Havu, V. Havu, X. Ren, K. Reuter, and M. Scheffler, *Comput. Phys. Commun.* **180**, 2175 (2009).
- <sup>2</sup> H. N. Rojas, R. W. Godby, and R. J. Needs, *Phys. Rev. Lett.* **74**, 1827 (1995).
- <sup>3</sup> J. Wilhelm, D. Golze, L. Talirz, J. Hutter, and C. A. Pignedoli, *J. Phys. Chem. Lett.* **9**, 306 (2018).
- <sup>4</sup> J. Wilhelm, P. Seewald, and D. Golze, *J. Chem. Theory Comput.* **17**, 1662 (2021).
- <sup>5</sup> Y. Jung, A. Sodt, P. M. W. Gill, and M. Head-Gordon, *Proc. Natl. Acad. Sci. U.S.A.* **102**, 6692 (2005).
- <sup>6</sup> A. Luenser, H. F. Schurkus, and C. Ochsenfeld, *J. Chem. Theory Comput.* **13**, 1647 (2017).
- <sup>7</sup> W. Kohn, *Phys. Rev. Lett.* **76**, 3168 (1996).
- <sup>8</sup> R. M. Martin, L. Reining, and D. M. Ceperley, *Interacting electrons* (Cambridge University Press, 2016).
- <sup>9</sup> T. Zhu and G. K.-L. Chan, *J. Chem. Theory Comput.* **17**, 727 (2021).
- <sup>10</sup> M. Guidon, J. Hutter, and J. VandeVondele, *J. Chem. Theory Comput.* **5**, 3010 (2009).
- <sup>11</sup> H. J. Monkhorst and J. D. Pack, *Phys. Rev. B* **13**, 5188 (1976).
- <sup>12</sup> K. Laughon, J. M. Yu, and T. Zhu, *J. Phys. Chem. Lett.* **13**, 9122 (2022).
- <sup>13</sup> P. Liu, M. Kaltak, J. Klimeš, and G. Kresse, *Phys. Rev. B* **94**, 165109 (2016).
- <sup>14</sup> D. Golze, M. Dvorak, and P. Rinke, *Front. Chem.* **7**, 377 (2019).
- <sup>15</sup> T. D. Kühne, M. Iannuzzi, M. Del Ben, V. V. Rybkin, P. Seewald, F. Stein, T. Laino, R. Z. Khaliullin, O. Schütt, F. Schiffmann, D. Golze, J. Wilhelm, S. Chulkov, M. H. Bani-Hashemian, V. Weber, U. Borštnik, M. Taillefumier, A. S. Jakobovits, A. Lazzaro, H. Pabst, T. Müller, R. Schade, M. Guidon, S. Andermatt, N. Holmberg, G. K. Schenter, A. Hehn, A. Bussy, F. Belleflamme, G. Tabacchi, A. Glöß, M. Lass, I. Bethune, C. J. Mundy, C. Plessl, M. Watkins, J. VandeVondele, M. Krack, and J. Hutter, *J. Chem. Phys.* **152**, 194103 (2020).
- <sup>16</sup> <https://github.com/cp2k/cp2k>.
- <sup>17</sup> S. Goedecker, M. Teter, and J. Hutter, *Phys. Rev. B* **54**, 1703 (1996).
- <sup>18</sup> F. Weigend, M. Häser, H. Patzelt, and R. Ahlrichs, *Chem. Phys. Lett.* **294**, 143 (1998).
- <sup>19</sup> [https://github.com/JWilhelm/Inputs\\_outputs\\_low\\_scaling\\_GW\\_TMDC](https://github.com/JWilhelm/Inputs_outputs_low_scaling_GW_TMDC).
- <sup>20</sup> Libint, A library for the evaluation of molecular integrals of operators over Gaussian functions, “<https://github.com/evaleev/libint>.”
- <sup>21</sup> D. Golze, N. Benedikter, M. Iannuzzi, J. Wilhelm, and J. Hutter, *J. Chem. Phys.* **146**, 034105 (2017).
- <sup>22</sup> J. Wilhelm, P. Seewald, M. Del Ben, and J. Hutter, *J. Chem. Theory Comput.* **12**, 5851 (2016).
- <sup>23</sup> P. Seewald, *Low-Scaling Electronic Structure Methods Based on Sparse Tensor Contraction*, Ph.D. thesis, University of Zurich (2021).
- <sup>24</sup> P. Giannozzi, O. Andreussi, T. Brumme, O. Bunau, M. B. Nardelli, M. Calandra, R. Car, C. Cavazzoni, D. Ceresoli, M. Cococcioni, N. Colonna, I. Carnimeo, A. D. Corso, S. de Gironcoli, P. Delugas, R. A. DiStasio, A. Ferretti, A. Floris, G. Fratesi, G. Fugallo, R. Gebauer, U. Gerstmann, F. Giustino, T. Gorni, J. Jia, M. Kawamura, H.-Y. Ko, A. Kokalj, E. Küçükbenli, M. Lazzeri, M. Marsili, N. Marzari,

- F. Mauri, N. L. Nguyen, H.-V. Nguyen, A. O. de-la Roza, L. Paulatto, S. Poncé, D. Rocca, R. Sabatini, B. Santra, M. Schlipf, A. P. Seitsonen, A. Smogunov, I. Timrov, T. Thonhauser, P. Umari, N. Vast, X. Wu, and S. Baroni, *J. Phys. Condens. Matter* **29**, 465901 (2017).
- <sup>25</sup> J. P. Perdew, K. Burke, and M. Ernzerhof, *Phys. Rev. Lett.* **77**, 3865 (1996).
- <sup>26</sup> M. J. van Setten, M. Giantomassi, E. Bousquet, M. J. Verstraete, D. R. Hamann, X. Gonze, and G.-M. Rignanese, *Comput. Phys. Commun.* **226**, 39 (2018).
- <sup>27</sup> M. S. Hybertsen and S. G. Louie, *Phys. Rev. B* **34**, 5390 (1986).
- <sup>28</sup> J. Deslippe, G. Samsonidze, D. A. Strubbe, M. Jain, M. L. Cohen, and S. G. Louie, *Comput. Phys. Commun.* **183**, 1269 (2012).
- <sup>29</sup> F. H. da Jornada, D. Y. Qiu, and S. G. Louie, *Phys. Rev. B* **95**, 035109 (2017).
- <sup>30</sup> S. Ismail-Beigi, *Phys. Rev. B* **73**, 233103 (2006).
- <sup>31</sup> P. Lazic, *Comput. Phys. Commun.* **197**, 324 (2015).
- <sup>32</sup> D. S. Koda, F. Bechstedt, M. Marques, and L. K. Teles, *J. Phys. Chem. C* **120**, 10895 (2016).
- <sup>33</sup> S. Carr, S. Fang, and E. Kaxiras, *Nat. Rev. Mater.* **5**, 748 (2020).
- <sup>34</sup> O. Vahtras, J. Almlöf, and M. Feyereisen, *Chem. Phys. Lett.* **213**, 514 (1993).
- <sup>35</sup> J. VandeVondele and J. Hutter, *J. Chem. Phys.* **127**, 114105 (2007).
- <sup>36</sup> S. Kundu, T. Amit, H. R. Krishnamurthy, M. Jain, and S. Refaely-Abramson, arXiv: 2209.05030 (2022).
- <sup>37</sup> D. Y. Qiu, F. H. da Jornada, and S. G. Louie, *Phys. Rev. B* **93**, 235435 (2016).
